# Supplementary material for: DISCO: A Hierarchical Disentangled Cognitive Diagnosis Framework for Interpretable Job Recommendation
Source: arXiv:2410.07671 source file (2024-10-15)
Supplement: Supplementary file 1 [file 8-appendix.tex]

\begin{table*}[!htbp]
\centering
\caption{Quantitative results on students score prediction.}
\begin{tabular}{c c | c c | c c | c c}
\toprule
% Datasets & Metrics & IRT(\%) & CA\_IRT(\%) & MIRT(\%) & CA\_MIRT(\%) & NCD(\%) &CA\_NCD(\%)
% Datasets & Methods & ACC($\uparrow$) & AUC($\uparrow$) & RMSE($\downarrow$) & NLL($\downarrow$) & BS($\downarrow$) &ECE($\downarrow$)
\textbf{Datasets} & \textbf{Metrics} & \textbf{IRT} & \textbf{Reli-IRT} & \textbf{MIRT} &\textbf{Reli-MIRT} & \textbf{NCD} & \textbf{Reli-NCD}

\\
% \hline
\midrule
\midrule
 \multirow{6}{*}{Assist09} & ACC~(\% $\uparrow$) &  &  &  &  &  & 
\\
~& RMSE~($\downarrow$)  &  &   &   &  &  & 
\\
~& AUC~(\% $\uparrow$)  &  &  &  &  & & 
\\
~& ECE~(\% $\downarrow$)  &  &  &  &  &  & 
\\
~& MCE~(\% $\downarrow$)  &  &  &  &  &   & 
\\
\midrule
 \multirow{6}{*}{e-Math} & ACC~(\% $\uparrow$) &  &  &  &  &  & 
\\
~& RMSE~($\downarrow$)  &  &   &   &  &  & 
\\
~& AUC~(\% $\uparrow$)  &  &  &  &  & & 
\\
~& ECE~(\% $\downarrow$)  &  &  &  &  &  & 
\\
~& MCE~(\% $\downarrow$)  &  &  &  &  &   & 
\\
\midrule
 \multirow{6}{*}{Junyi} & ACC~(\% $\uparrow$) &  &  &  &  &  & 
\\
~& RMSE~($\downarrow$)  &  &   &   &  &  & 
\\
~& AUC~(\% $\uparrow$)  &  &  &  &  & & 
\\
~& ECE~(\% $\downarrow$)  &  &  &  &  &  & 
\\
~& MCE~(\% $\downarrow$)  &  &  &  &  &   & 
\\
\midrule
 \multirow{6}{*}{ENEM} & ACC~(\% $\uparrow$) &  &  &  &  &  & 
\\
~& RMSE~($\downarrow$)  &  &   &   &  &  & 
\\
~& AUC~(\% $\uparrow$)  &  &  &  &  & & 
\\
~& ECE~(\% $\downarrow$)  &  &  &  &  &  & 
\\
~& MCE~(\% $\downarrow$)  &  &  &  &  &   & 
\\
\bottomrule
\vspace{1mm}
\end{tabular}\label{tab2}
\end{table*}

\begin{table*}[!htbp]
	\centering
	\caption{A list of main notations used in this paper.}
	\begin{tabular}{c|l}
		\hline
		Nota. & Description  \\
		\noalign{\smallskip}\hline\noalign{\smallskip}
            $N$ & the number of students
            \\
             $M$ & the number of exercises
            \\
             $K$ & the  number of knowledge concepts
            \\
            $x_i^s$ & the one-hot encoded representation of student $s_i$
            \\
            $x_j^e$ & the one-hot encoded representation of exercise $e_j$
            \\
            $\mu_i$, $\sigma_i$ & the mean and the variance of student $s_i$, respectively
            \\
            $q(z_i|x_i^s)$ & the gaussian distribution of student $s_i$
            \\
            $\theta_i$ & the ability representation of student $s_i$
            \\
            $d$ & the dimensionality of ability representation of student $s_i$. For MIRT and NCD, d = K. For IRT, d=1
            \\
             $h_j^{diff}, h_j^{disc}$ & the difficulty and the discrimination of exercise $e_j$, respectively
            \\
             $p_{\phi}(z_i)$ &  the prior distribution for the ability status of student $s_i$
            \\
            $q_{\varphi} (z_i | x_i)$ & the posterior distribution of student $s_i$
            \\
            $\log p(r_{ij}|z_i)$ &  the likelihood of student $s_i$ answering correctly in exercise $e_j$
            \\
            $o_{ik}$ &   the proportion of the frequency of correct predictions of $s_i$ on concept $c_k$
            \\
            \noalign{\smallskip}\hline\noalign{\smallskip}
	\end{tabular}
\end{table*}

\begin{table*}[!htbp]
\centering
\caption{Results of Reli-NCD and its variants.}
\begin{tabular}{c c  c c  c c c}
\toprule
\textbf{Datasets} & \textbf{Mothod} & \textbf{ACC} & \textbf{RMSE} & \textbf{AUC} &\textbf{ECE} & \textbf{MCE} 
\\
\midrule
\midrule
 \multirow{3}{*}{Assist09} & w/o pre-train & 0.726778 & 0.432351 & 0.750200 & 0.041657 &  0.055882
\\
~& w/o ranking loss  &  0.729880 & 0.430568 & 0.753297  & 0.039767 & 0.078497
\\
~& Reli-NCD  & 0.730584 & 0.430039 & 0.754113 & 0.019367 & 0.050134
\\
\midrule
\multirow{3}{*}{e-Math} &   w/o pre-train & 0.691121 & 0.439397 & 0.739707 & 0.024114 & 0.045883
\\
~& w/o ranking loss  & 0.692634 & 0.439983 & 0.739693 & 0.028616 & 0.062537
\\
~& Reli-NCD  & 0.693889 & 0.438941  & 0.740297 & 0.014149 & 0.023308 
\\
\midrule
 \multirow{3}{*}{Junyi} &  w/o pre-train  & 0.758085 & 0.405946 & 0.799368 & 0.017816 & 0.031330
\\
~& w/o ranking loss  & 0.760339 & 0.405310 & 0.799828  & 0.017047 & 0.031460
\\
~& Reli-NCD  & 0.763038  & 0.402801  & 0.802150 & 0.006040 & 0.012843
\\
\midrule
 \multirow{3}{*}{ENEM} & w/o pre-train & 0.733781  & 0.428751  & 0.728521 & 0.008946 & 0.016452
\\
~& w/o ranking loss  & 0.734549 & 0.428644 & 0.728227 & 0.009453 & 0.012280
\\ 
~& Reli-NCD  & 0.734392 & 0.428586  & 0.728256 &  0.005620 & 0.011819 
\\
\bottomrule
\vspace{1mm}
\end{tabular}\label{tab2}
\end{table*}

\begin{table*}[!htbp]
\centering
\caption{Impact of different sizes of $\gamma$ on the performance.}
\begin{tabular}{c c  c c  c c c}
\toprule
\textbf{Datasets} & \textbf{$\gamma$} & \textbf{ACC} & \textbf{RMSE} & \textbf{AUC} &\textbf{ECE} & \textbf{MCE} 
\\
\midrule
\midrule
 \multirow{6}{*}{Assist09} & 1 & 0.687765 & 0.453169 & 0.687300 & 0.043167 &  0.071312
\\
~& 1e-1  &  0.692523  & 0.448774  &  0.700456 & 0.034146 & 0.060494
\\
~& 1e-2  & 0.712809 & 0.439906 & 0.735297  & 0.047236  & 0.064088
\\
~& 1e-3  & 0.727558 & 0.433149 & 0.750142 & 0.048140 & 0.083792
\\
~& 1e-4  & 0.729385 & 0.432970 & 0.752284 & 0.054166 & 0.094093
\\
~& 1e-5  & 0.731060 & 0.433350 & 0.753912 & 0.059409 & 0.104707
\\
~& 1e-6  & 0.728034 & 0.430124 & 0.752707 & 0.022477 & 0.090163
\\
\midrule
 \multirow{6}{*}{e-Math} & 1 & 0.678439 & 0.451492  & 0.704254 & 0.018133 &  0.045946
\\
~& 1e-1  & 0.682546  & 0.449353 & 0.710574   & 0.007373 & 0.016879 
\\
~& 1e-2  & 0.687474 & 0.442277  & 0.733318  & 0.015883 & 0.029616 
\\
~& 1e-3  & 0.691170 & 0.440786 & 0.740498  & 0.029325 & 0.046571
\\
~& 1e-4  & 0.691889 & 0.439941 & 0.740297 & 0.014149 & 0.023308 
\\
~& 1e-5  & 0.687988 & 0.439221 & 0.743523 & 0.025969 & 0.034162 
\\
~& 1e-6  & 0.690349 &  0.439675 & 0.742888 & 0.025869 & 0.035111 
\\
\midrule
 \multirow{6}{*}{Junyi} & 1 & 0.734857 & 0.419867 & 0.766009 & 0.007257 &  0.014334
\\
~& 1e-1  &  0.739587 & 0.417555 &  0.769867 & 0.011138 & 0.013716
\\
~& 1e-2  & 0.748106 & 0.412579 & 0.782208 & 0.012902 & 0.031133 
\\
~& 1e-3  & 0.763038 & 0.402801 & 0.802150 & 0.006040 & 0.012843
\\
~& 1e-4  & 0.762914 & 0.402539 & 0.802355 & 0.008547 & 0.017398
\\
~& 1e-5  & 0.763583 & 0.402591 & 0.803423 & 0.007876 & 0.011836
\\
~& 1e-6  & 0.763483  & 0.402691 & 0.803423 & 0.015645 & 0.028991
\\
\midrule
 \multirow{6}{*}{Enem} & 1 & 0.699568  & 0.445792 & 0.683704 & 0.015735 &  0.028201 
\\
~& 1e-1  & 0.701119  & 0.445588 &  0.684706 & 0.014474 & 0.030838 
\\
~& 1e-2  & 0.710105  & 0.442126 & 0.694419 & 0.012019 & 0.058186 
\\
~& 1e-3  & 0.732243 & 0.429659 & 0.726869 & 0.011629 & 0.015166 
\\
~& 1e-4  & 0.734392 & 0.428586  & 0.728256 & 0.005620 & 0.011819 
\\
~& 1e-5  & 0.734411  & 0.428646 & 0.728203 &  0.006786 & 0.010155
\\
~& 1e-6  & 0.733716 &  0.428895 & 0.728526 & 0.009075 &  0.009075
\\
\bottomrule
\vspace{1mm}
\end{tabular}\label{tab2}
\end{table*}

\begin{table*}[!htbp]
\centering
\caption{Impact of different sizes of $\beta$ on the performance.}
\begin{tabular}{c c  c c  c c c}
\toprule
\textbf{Datasets} & \textbf{$\beta$} & \textbf{ACC} & \textbf{RMSE} & \textbf{AUC} &\textbf{ECE} & \textbf{MCE} 
\\
\midrule
\midrule
 \multirow{6}{*}{Assist09} & 1 & 0.725522 & 0.432134 & 0.750085 & 0.034049 &  0.067108
\\
~& 1e-1  & 0.725313  & 0.431429 & 0.747820  & 0.014521 & 0.039091
\\
~& 1e-2  & 0.730165 & 0.431237 & 0.753077 & 0.045912 & 0.077940
\\
~& 1e-3  & 0.732335 & 0.431530 & 0.755276 & 0.054878 & 0.097183
\\
~& 1e-4  & 0.731155 & 0.431585 & 0.753562 & 0.043300 & 0.091115
\\
~& 1e-5  & 0.729937 & 0.431408 & 0.753177 & 0.046312 & 0.086130
\\
~& 1e-6  & 0.729994 & 0.430964 & 0.753300 & 0.043945 & 0.079912
\\
\midrule
 \multirow{6}{*}{e-Math} & 1 & 0.691889 & 0.439830 & 0.739440 & 0.024103 &  0.047632
\\
~& 1e-1  &  0.690965 & 0.440099  & 0.738761  & 0.025455 &  0.047885 
\\
~& 1e-2  & 0.690965 & 0.439447 & 0.738889 & 0.018000 & 0.027943 
\\
~& 1e-3  & 0.691581 & 0.439421 & 0.739384 & 0.022305 & 0.040544
\\
~& 1e-4  & 0.690862 & 0.439481 & 0.739768 & 0.025495 & 0.039974 
\\
~& 1e-5  & 0.691889 & 0.439581 & 0.738041  & 0.015506 & 0.025788 
\\
~& 1e-6  & 0.692813 & 0.439446 & 0.739119 &  0.018094 & 0.036153 
\\
\midrule
 \multirow{6}{*}{Junyi} & 1 & 0.760116 & 0.404620 &  0.799335 & 0.009820 &  0.016394
\\
~& 1e-1  & 0.759868  & 0.404977 &  0.799666 & 0.006471 &  0.017713
\\
~& 1e-2  & 0.758680 & 0.405397 & 0.798936 & 0.008564 & 0.018462
\\
~& 1e-3  & 0.760215 & 0.405063 & 0.799679 & 0.010032 & 0.021795
\\
~& 1e-4  & 0.760116 & 0.405414 & 0.799719 & 0.016113 & 0.035213
\\
~& 1e-5  & 0.758234 & 0.405715 & 0.799574 & 0.011885 & 0.019553
\\
~& 1e-6  & 0.759769 & 0.405349 & 0.798712 & 0.007232 & 0.018847
\\
\midrule
 \multirow{6}{*}{Enem} & 1 & 0.733900 & 0.428786 & 0.728006 & 0.008972 &  0.020250 
\\
~& 1e-1  &  0.733454 & 0.429047 &  0.728480 & 0.009654 & 0.011296 
\\
~& 1e-2  & 0.734630 & 0.428515 & 0.728389 & 0.006985 & 0.010104
\\
~& 1e-3  &  0.734819 & 0.428502 & 0.728800 & 0.008828 & 0.015067 
\\
~& 1e-4  & 0.734781 & 0.428510 &  0.728847 & 0.004805 & 0.012200 
\\
~& 1e-5  & 0.735146 & 0.428386 & 0.728906 & 0.005388 & 0.010516
\\
~& 1e-6  & 0.734746 & 0.428541 & 0.728582 & 0.005317 & 0.007748 
\\
\bottomrule
\vspace{1mm}
\end{tabular}\label{tab2}
\end{table*}
